# Supplementary material for: Learning context-aware adaptive solvers to accelerate quadratic programming
Source: arXiv:2211.12443 source file (2022-11-22)
Supplement: Supplementary file 1 [file ADMM_MDP.tex]

In this section, we provide the ADMM algorithm's internal process. \\
If actor $\pi$ generates $\rho_t$ with input $x_t, \mC_t$, the action $\rho_t$ is assigned to ADMM’s penalty parameter $\rho$. With the new penalty parameter $\rho_t$, ADMM iterations are performed in a default fixed number $10$.\\
Suppose primal and dual residual terms satisfy termination conditions earlier than $10$ iterations. In that case, it ends immediately, and the environment provides the last state $x_{t}$ and reward $r_{t}$.\\
If residual terms do not satisfy termination conditions during $10$ iterations, QP env provides next state $x_{t+1}$ and reward $r_{t}$, and actor generates action $\rho_{t+1}$ depend on state $x_{t+1}$.

% \begin{algorithm}[H]
% 	\caption{QP's internal process at time step $t$}
% 	\label{alg:QP_step_function}
% 	\hspace*{\algorithmicindent} \textbf{Input} state $x_t$, action $\rho_t$, QP env \\
% 	\hspace*{\algorithmicindent} \textbf{Output} next state $x_{t+1}$, $\texttt{done}_t$, reward $r_t$ 
% 	\begin{algorithmic}[1]
% 	    \State $r_t \gets 0, x_{t}^{0} \gets x_{t}$
% 	    % QP env recieve action $\rho_{t}$ at timestep $t$
% 		\For {$i \in \{0, 1, 2,\ldots, 9\} $}
% 		    \State Conduct an ADMM iteration with $\rho_{t}$ at $x_{t}^{i}$
% 			\State Generate intermediate $x_{t}^{i+1}$ from $x_t^i$ and QP env
% 			\State Calculate residual norm $||r^{\text{primal}}||_{\infty}$, $||r^{\text{dual}}||_{\infty}$ 
%             \State Calculate tolerances $\epsilon^{\text{primal}}$, $\epsilon^{\text{dual}}$ 
% 			\If {$||r^{\text{primal}}||_{\infty} < \epsilon^{\text{primal}}$  and $||r^{\text{dual}}||_{\infty} < \epsilon^{\text{dual}}$}
% 			    \State $\texttt{done}_t \gets 1$ 
% 			    \State \textbf{break}
%             \Else
%                 \State $\texttt{done}_t \gets 0$
%                 \State $r_{t} \gets r_{t} -1$
%     		\EndIf
% 		\EndFor
% 		\State $x_{t+1} = x^{i}_{t}$ \\
% 		\Return $x_{t+1}, r_{t}, \texttt{done}_t$
% 	\end{algorithmic} 
% \end{algorithm}
