# Supplementary material for: Learning context-aware adaptive solvers to accelerate quadratic programming
Source: arXiv:2211.12443 source file (2022-11-22)
Supplement: Supplementary file 2 [file Graph_preprocess_const.tex]

% \usepackage{algorithm}
% \usepackage{algpseudocode}

% \algdef{SE}[SUBALG]{Indent}{EndIndent}{}{\algorithmicend\ }%
% \algtext*{Indent}
% \algtext*{EndIndent}

% \usepackage{algorithm}% http://ctan.org/pkg/algorithm
% \usepackage{algpseudocode}%

% \begin{algorithm}
% 	\caption{matrix scaling at constraints} \label{alg:constraint_scaling}
% 	\begin{algorithmic}[1]
% 		\For {$j = 1, 2,\ldots, M $} \Comment{$M$ is number of constraints}
% 		    \State Calculate $A^{*}_{j}$, maximum constraint term for constraint $j$
% 	        \Indent
%                 \State $A^{*}_{j} := \max_{i}(|A_{ji}|)$
%             \EndIndent
%             \State Calculate scaled $A_{ji}^{new}, u_{j}^{new}, l_{j}^{new}$
%             \State $A^{new}_{ji} = \frac{A_{ji}}{A^*_j} \qquad  i = 1, 2, \ldots, N $ \Comment{$N$ is dimension of variable $x$}
%             \State $u^{new}_{j} = \frac{u_j}{A^*_j}$ 
%             \State $l^{new}_j = \frac{l_j}{A^*_j}$
% 		\EndFor
% 		\State Generate scaled matrices $A^{new}, u^{new}, l^{new}$
% 		\Indent
%     		\State $[A^{new}]_{ji} = A^{new}_{ji} \qquad \forall i, j $
%     		\State $[u^{new}]_j = u^{new}_{j}  \qquad \forall j $
%     		\State $[l^{new}]_j = l^{new}_{j}  \qquad \forall j $
% 		\EndIndent
% 	\end{algorithmic} 
% \end{algorithm}     
