# Supplementary material for: Learning context-aware adaptive solvers to accelerate quadratic programming
Source: arXiv:2211.12443 source file (2022-11-22)
Supplement: Supplementary file 3 [file Graph_preprocess_obj.tex]

% \begin{algorithm}
% \caption{matrix scaling at the objective function} \label{alg:objective_scaling}
% 	\begin{algorithmic}[1]
% 		\State Assume the objective function $x^{T}Px + q^Tx$
% 		\State Calculate maximum objective term $P^{*}$
% 		\Indent
% 	        \State $P^*_{diag} := \max_{i}|P_{ii}|$
% 	        \State $P^*_{non-diag} := 2* \max_{i, j, i\neq j} |P_{ij}|$
%             \State $P^* := \max(P^*_{diag}, P^*_{non-diag}) $
%         \EndIndent
%         \State Calculate scaled matrices $P^{new}, q^{new}$
%         \Indent
%             \State $P^{new} := \frac{P}{P^*}$
%             \State $q^{new} := \frac{q}{P^*}$
%         \EndIndent
% 	\end{algorithmic} 
% \end{algorithm}
