# Supplementary material for: Learning context-aware adaptive solvers to accelerate quadratic programming
Source: arXiv:2211.12443 source file (2022-11-22)
Supplement: Supplementary file 4 [file context_encoder.tex]

% \subsection{Model architecture}
In this section, we provide the detail architecture of the context encoder. The context encoder is composed of 'spatial' and 'temporal' parts. Spatial and temporal parts consists of the HGA and GRU network, respectively. 

\paragraph{Spatial context encoder structure}

\paragraph{Temporal context encoder structure}
